# Supplementary material for: Inferring fine-grained migration patterns across the United States
Source: arXiv:2503.20989 source file (2026-01-07)
Supplement: Supplementary file 2 [file A1_validations.tex]

\section{Additional details on validations}
\label{SI:validation}

Here we provide additional details on \ourdataset validations. We include additional details on our held-out data validations; a semi-synthetic data validation where we verify our method reconstructs a known ground-truth matrix; details on related work documenting biases of Infutor, which is the subject of our Figure \ref{fig:biases}; and additional socioeconomic and demographic dimensions on which we assessed biases, including undocumented immigrants.

\subsection{Validating the estimation procedure using held-out data}
\label{SI:validation-heldout}

\begin{table}[htbp]
\centering
\begin{subtable}{\textwidth}
\centering
\begin{tabular}{r|l|c|c|c|}
\multicolumn{2}{c|}{} & \textbf{\ourdataset} & \textbf{CBG Held-Out} & \textbf{State Held-Out} \\
\hline
\multirow{4}{*}{\textbf{Population counts}} 
& State & 1.000 & 1.000 & 1.000 \\
& County & 1.000 & 1.000 & 1.000 \\
& Tract & 0.997 & 0.888 & 0.998 \\
& CBG & 0.996 & 0.856 & 0.997 \\
\hline
\multirow{2}{*}{\textbf{Population flows}} 
& State & 1.000 & 1.000 & 1.000 \\
& County & 1.000 & 1.000 & 1.000 \\
\hline
\multirow{2}{*}{\textbf{Population flows (area movers only)}} 
& State & 0.998 & 0.998 & 0.895 \\
& County & 0.957 & 0.956 & 0.949 \\
\hline
\multirow{2}{*}{\textbf{Population flows (area stayers only)}} 
& State & 1.000 & 1.000 & 1.000 \\
& County & 1.000 & 1.000 & 1.000 \\
\hline
\multirow{2}{*}{\textbf{In-migration}} 
& State & 0.998 & 0.998 & 0.885 \\
& County & 0.984 & 0.983 & 0.963 \\
\hline
\multirow{2}{*}{\textbf{In-migration rate}} 
& State & 0.987 & 0.987 & 0.663 \\
& County & 0.715 & 0.705 & 0.629 \\
\hline
\end{tabular}
\caption{Pearson correlation between Census data  and our estimates with CBG and state data held out. Pearson correlations with \ourdataset, which is estimated using all data sources, are presented for comparison. As noted in the main text, perfect correlations between \ourdataset and all flows or stayers are partially driven by variation in area size and the predominance of non-mover counts among flows.}
\label{tab:validations_corr}
\end{subtable}

\begin{subtable}{\textwidth}
\centering
\begin{tabular}{r|l|c|c|c|}
\multicolumn{2}{c|}{} & \textbf{\ourdataset} & \textbf{CBG Held-Out} & \textbf{State Held-Out} \\
\hline
\multirow{4}{*}{\textbf{Population counts}} 
& State & 100.00 & 100.00 & 100.00 \\
& County & 100.00 & 100.00 & 100.00 \\
& Tract & 85.88 & 13.46 & 88.13 \\
& CBG & 83.60 & 9.08 & 85.09 \\
\hline
\multirow{2}{*}{\textbf{Population flows}} 
& State & 89.46 & 89.40 & 80.87 \\
& County & 90.65 & 90.70 & 75.24 \\
\hline
\multirow{2}{*}{\textbf{Population flows (area movers only)}} 
& State & 87.46 & 87.06 & 4.08 \\
& County & 42.34 & 41.30 & 4.65 \\
\hline
\multirow{2}{*}{\textbf{Population flows (area stayers only)}} 
& State & 89.46 & 89.40 & 81.03 \\
& County & 91.01 & 91.08 & 75.59 \\
\hline
\multirow{2}{*}{\textbf{In-migration}} 
& State & 90.93 & 91.11 & 7.22 \\
& County & 68.92 & 68.19 & 6.55 \\
\hline
\multirow{2}{*}{\textbf{In-migration rate}} 
& State & 87.30 & 87.33 & 4.89 \\
& County & 51.75 & 50.91 & 0.73 \\
\hline
\end{tabular}
\caption{Reductions in RMSE. We compute RMSE between (1) our estimates and Census data and (2) Infutor data and Census data, and report the reduction in RMSE from using our estimates. Positive values indicate improvements. Values are average reductions across all years with overlapping ground-truth data releases.}
\label{tab:validations_RMSE}
\end{subtable}
\caption{Validation of estimates in held-out data settings. The full model validations are repeated for comparison. For in-migration rates, metrics are weighted by populations to account for disparate county and state sizes.}
\label{tab:validations}
\end{table}

We verify that our estimation procedure yields highly correlated estimates with each Census data source even when it is removed from the datasets used for estimation. For example, we remove CBG-level Census populations from our estimation datasets, and verify that our resulting estimates remain highly correlated with CBG-level data. Specifically, we conduct our full battery of validations on two additional sets of migration estimates: ``CBG held-out'', which is estimated without the CBG-level population data (i.e. $\rawinfutormatrix^{(t)}$ was not scaled to match ACS 5-year CBG populations); and ``State held-out'', which is estimated without the state-level flow data (i.e. $\rawinfutormatrix^{(t)}$ was not scaled to match ACS 1-year state-to-state flows nor state mobility rates). Supplementary Table \ref{tab:validations} reports values for the Pearson correlation across all estimates and ground-truth as well as relative error reduction from Infutor. Values for the original \ourdataset estimates, reported in Figure \ref{fig:validations}, are reproduced for easy comparison.

The CBG held-out and State held-out estimates remain highly correlated with all Census datasets ($\rho$ above $0.629$); they also reduce RMSE relative to Infutor. Unsurprisingly, both the correlations and error reductions are smaller than those achieved by our full \ourdataset estimates, which make use of all sources of Census data. Together, these results illustrate both that (a) our estimation pipeline generalizes well to held-out data and that (b) all datasets used in the training help improve concordance with Census data, justifying their inclusion.

\subsection{Validating the harmonization procedure with semi-synthetic data}
\label{SI:validation-synthetic}

We further validate our harmonization procedure using semi-synthetic data, a standard check for statistical methods when ground-truth data is lacking \cite{balachandar2024domain, agostini2024bayesian, pierson2019inferring}. Specifically, we assess how well our harmonization procedure can recover a known CBG-to-CBG flow matrix, given only a perturbed version of that matrix and the same set of marginal constraints available in our main analysis (e.g., CBG-level populations). 

To generate realistic semi-synthetic data, we use the \ourdataset matrices as the ground-truth CBG-to-CBG flow matrices $M$, since these are likely more realistic than purely synthetic data generated from stylized models. These ground-truth matrices $M$ are not used as input to our harmonization method, but only as validation. From $M$, we produce the perturbed CBG-to-CBG flow matrix $\rawinfutormatrix$ by adding multiplicative noise; we describe this process further below. We also compute the same marginals of $M$ that are available in our main analysis: specifically, CBG populations; state-level counts of movers and non-movers; state-to-state flows; and county populations. We use these marginals and the perturbed matrix $\rawinfutormatrix$ as inputs to our harmonization method. We assess how well our method recovers the ground-truth matrix $M$ using the same metrics described in the main text (reduction in RMSE relative to using $\rawinfutormatrix$ alone, and Pearson correlation). 

To thoroughly test the robustness of our method, we consider two processes for generating $\rawinfutormatrix$ from $M$. We now describe these processes.

\paragraph{Harmonizing in the presence of structured multiplicative noise}

Our harmonization procedure assumes that the difference between the ground-truth matrix $M$ and the perturbed matrix $\rawinfutormatrix$ can be described by a series of multiplicative scalings with a given structure (e.g., CBG-level scalings on each row) as described in the Methods Section. We thus first test how well our harmonization procedure recovers the ground-truth matrix if the perturbation does indeed match that structure. Specifically, we draw independent Log-Normal random variables that multiply (1) each row of $M$ (mirrors CBG population fitting), (2) each group of diagonal entries within the same state (mirrors state non-movers fitting), (3) each group of off-diagonal entries in columns within the same state (mirrors state movers fitting), (4) each group of entries within the same state-to-state pair (mirrors state flows fitting) and (5) each group of rows within the same county, and each group of columns within the same county (mirrors county population fitting). We draw the Log-Normal noise using standard deviations $\tau$ ranging from $0.05$ to $0.20$. We choose the upper bound on this range because it exceeds the level of variation we observe in real-world data. Specifically, across states (Figure \ref{fig:biases}\textbf{a}), the biases between ground-truth and Infutor populations have standard deviation 0.11; across counties, the standard deviation is 0.19, both exceeded by our upper bound of $\tau = 0.20$. (We do verify, however, that results remain robust up to much larger $\tau$ values of 1.00).

We find that our harmonization method performs very strongly in this setting. For all standard deviations of noise, our inferred matrix achieves Pearson correlations above 0.99 either on the full CBG-CBG matrix or when restricting to CBG-CBG movers. The harmonized matrix also reduces RMSE (relative to the original perturbed matrix $\rawinfutormatrix$) by an average of 97.7\% across all years and noise levels (sd 0.06\%), and by 91.9\% when restricting to off-diagonal entries (sd 0.67\%). These RMSE reductions remain consistently strong across the range of noise scales. The small residual error is an expected result of the optimization procedure; for example, we only fit once to CBG-level marginals to avoid overfitting, so are not guaranteed to match these marginals. 

\paragraph{Harmonizing in the presence of real-world bias and independent noise}

We next assess the performance of our harmonization procedure when the perturbation does not match the structure it assumes, but consists both of real-world bias and independent noise. Specifically,  we produce the perturbed matrix $\rawinfutormatrix$ from $M$ as follows:
\[E_{ij} = M_{ij}\cdot \exp\left\{b\cdot\left(w_i + w_j\right) + \sigma \cdot Z_{ij}\right\}\]
where $w_i$ is the z-scored share of the white population in CBG $i$ (capturing real-world biases, as shown in Figure \ref{fig:biases}\textbf{c}) and $Z_{ij}$ are i.i.d. standard normal variables. The parameters $b$ and $\sigma$ control the relative scales of the bias and the independent noise, respectively. We assess performance across a range of $b$ and $\sigma$, choosing $b$ to represent a realistic level of real-world bias based on our results in Figure \ref{fig:biases}\textbf{c}, and noise scales $\sigma$ up to 0.20, as above. 

We would expect high levels of independent noise to make it very challenging to recover the off-diagonal entries of the ground-truth matrix. This is because the diagonal entries of the migration matrix are much bigger than the off-diagonal entries (since most people do not move); thus, the scaling factors learned by the harmonization procedure will be dominated by the diagonal entries. This is generally reasonable: if we want to estimate bias in the movers from a CBG, the bias of the entire CBG population likely serves as a good proxy. However, this logic fails under independent noise, since noise in the diagonals provides no information about noise in the off-diagonals. Importantly, the challenge of correcting for independent noise applies not just to our harmonization procedure, but to any correction procedure, since correcting such noise would require information about the ground truth for each entry.

\begin{figure}[h!]
	\centering
\includegraphics[width=\textwidth]{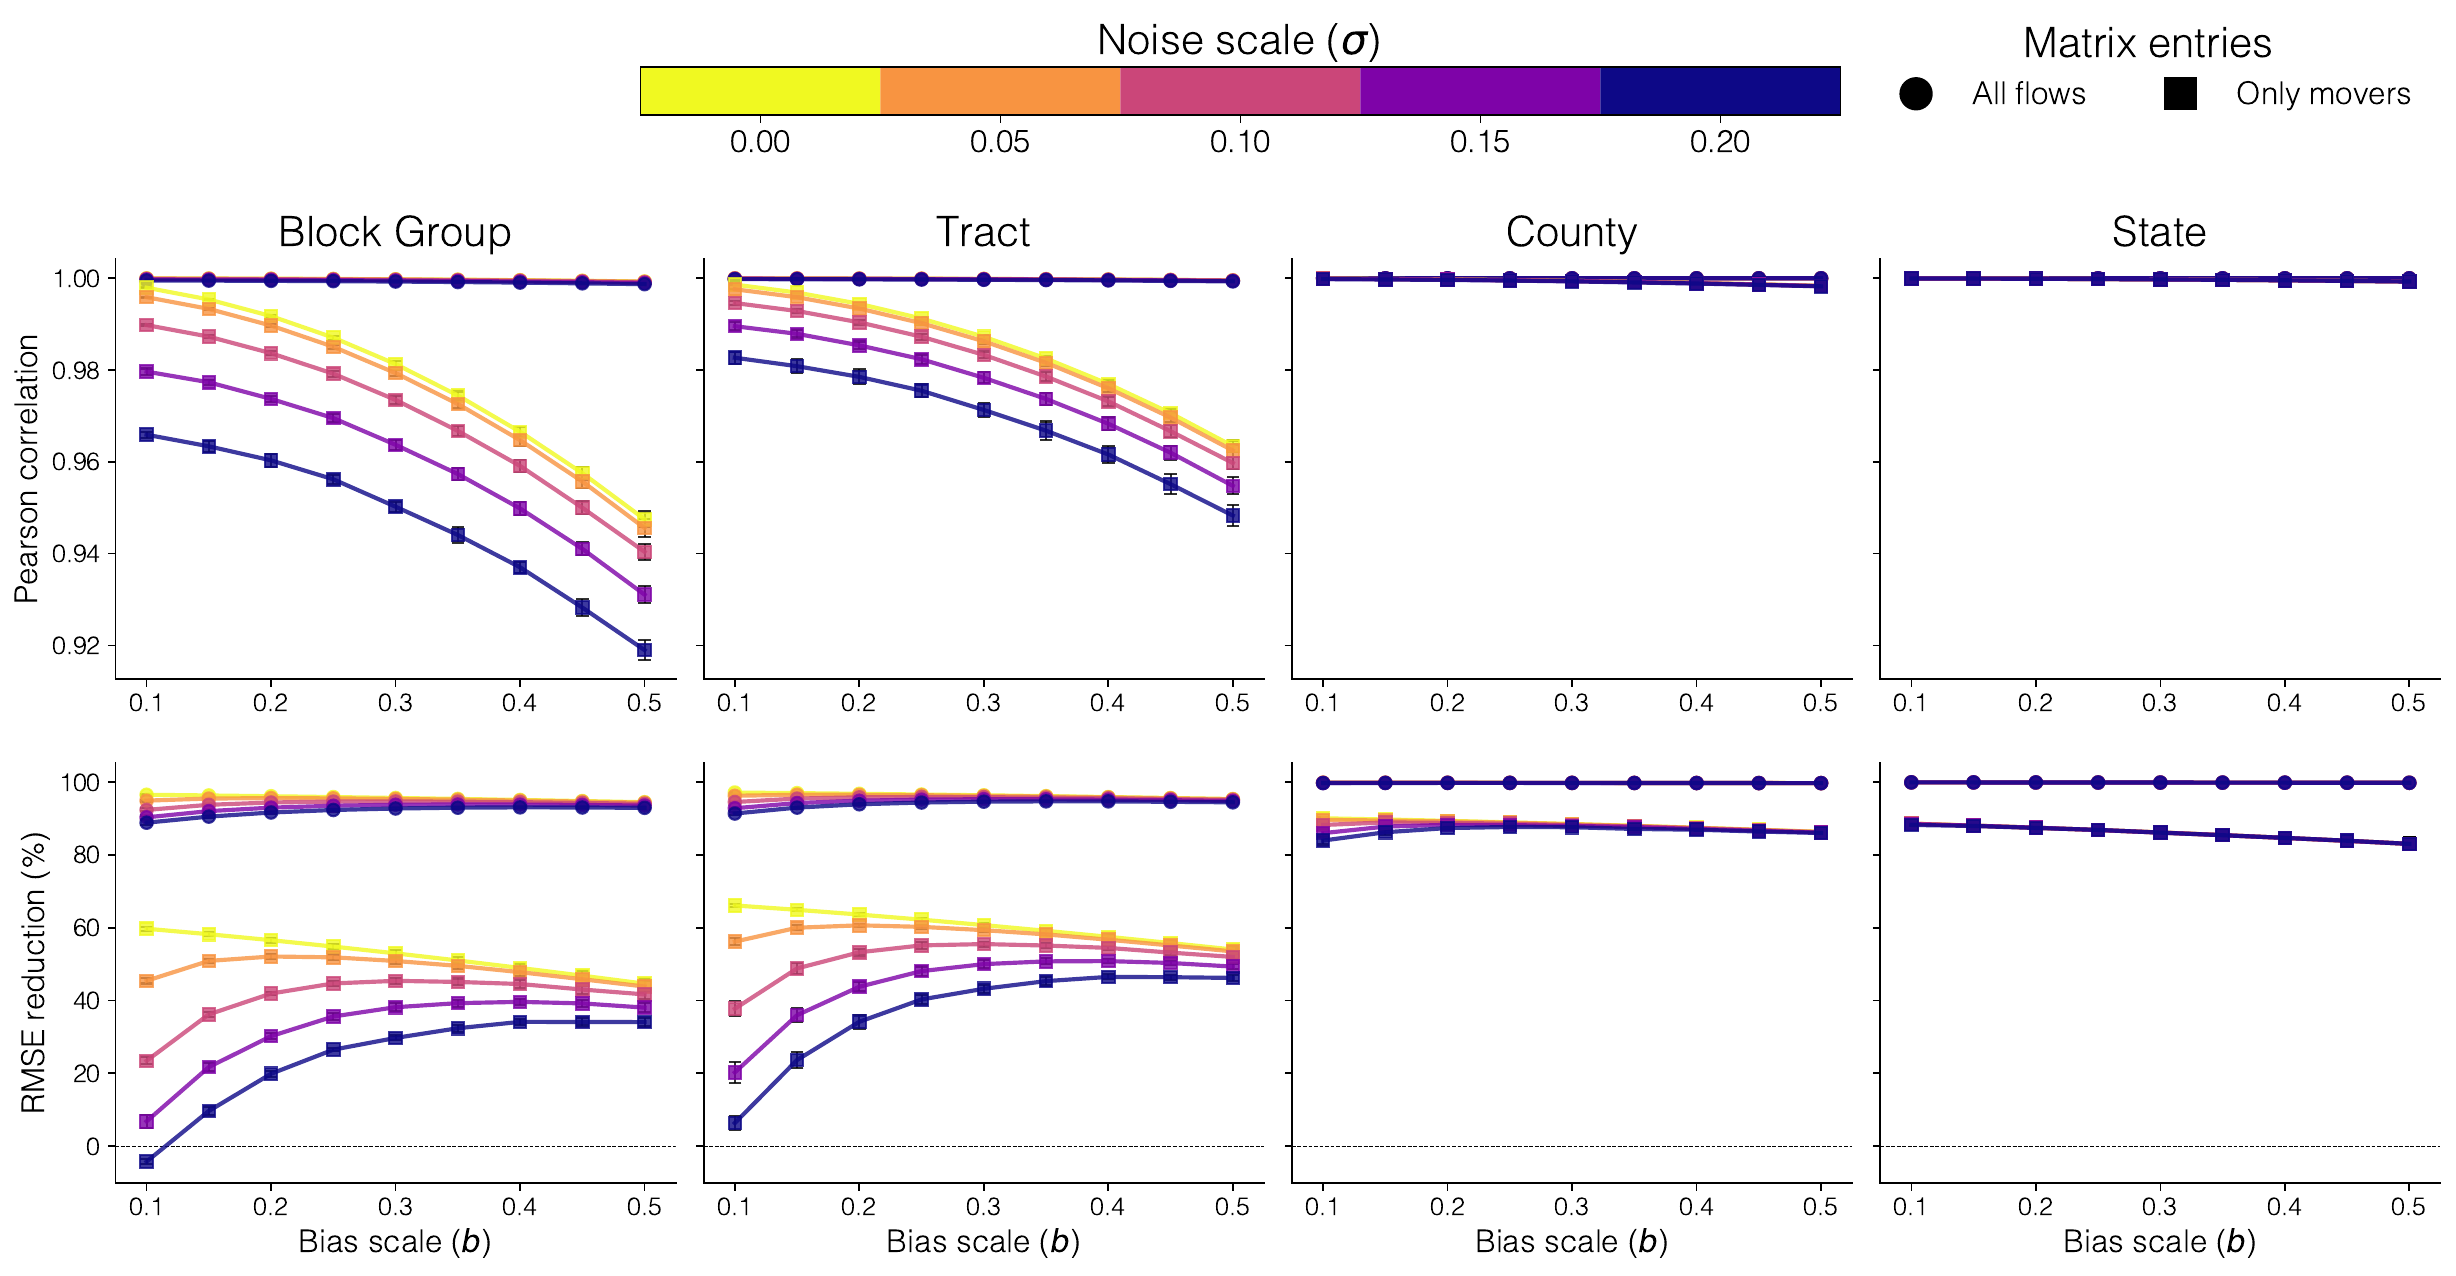}
	\caption{\textbf{Experimental validations of our method.} Pearson correlation and reduction in RMSE achieved by our harmonization procedure on semi-synthetic data with real-world bias and independent noise. We report average metrics across all years; error bars plot standard deviation across years (from 2010-11 to 2018-19, $n=9$). Circles represent metrics computed on all entries of the flow matrix; squares represent metrics computed on movers only (off-diagonal elements). Columns assess metrics for flows at the CBG level, tract level, county level, and state level. We assess results when varying the level of bias (x-axis) and independent noise (line color).}
    \label{fig:synthetic}
\end{figure}

Supplementary Figure \ref{fig:synthetic} plots the Pearson correlation and reduction in RMSE for flows at every geographic scale. We compute metrics with respect to all flows and movers only (off-diagonal entries) for varying levels of noise and bias. Results are consistent with the analysis above. When considering all flows (as opposed to just off-diagonal entries), error is reduced almost completely and correlations are nearly perfect at all geographic scales (circular points). When restricting to off-diagonal entries specifically (square points) on the more granular geographic scales (tract and CBG levels), we find the largest error reductions when the scale of the independent noise is not too large relative to the bias, as expected. Pearson correlations decrease as bias and noise increase, but remain relatively high (above $0.91$ in all cases). State and county-level metrics for movers remain robust at all noise and bias scales because we have better marginal data with which to correct them (including state-to-state movers and county populations).

Collectively, these synthetic experiments show that our harmonization procedure performs well in recovering the ground-truth matrix as long as the structure of the perturbation lies within the family it is able to estimate; in contrast, purely independent noise is unsurprisingly harder to correct (both for our procedure and for any correction procedure). The family of perturbations our harmonization procedure can estimate is highly flexible (due to the number of scalings of varying shapes it incorporates) and indeed more flexible than classic iterative proportional fitting, which is widely used in similar demographic applications \cite{birkin_synthesissynthetic_1988,wong_reliability_1992, simpson_combining_2005, chang2021mobility, chang2024inferring} and estimates only row and column-level scalings. The assumption that the perturbation is structured, as opposed to entirely independent for each entry, is also substantiated by our and previous findings of systematic demographic bias in Infutor data, which would not emerge under purely independent noise. %Additionally, we verified that at state level---for which we have yearly ACS flow estimates---the error in Infutor flow estimates is also significantly predicted by the state of origin (p-value \gabriel{p-val})\footnote{To test this hypothesis, we used an F-test. We regressed the yearly relative error of Infutor flows on state-of-origin indicator variables.}.

\subsection{Related work documenting biases in the Infutor data}
\label{SI:validation-biases}

Many authors have assessed bias in the Infutor dataset, generally focusing on the data subsets or demographic characteristics most relevant to their own analyses. To our knowledge, the analysis we present in Figure \ref{fig:biases} constitutes the first comprehensive documentation of biases in the Infutor dataset across (a) a long period of time and (b) the entire United States. We include here a non-exhaustive review of works with documentation of Infutor biases.

As we report in Table \ref{tab:INFUTOR_stats_detailed}, Infutor undercounts the national US population. This is consistent with prior work; a similar finding is reported by \citet{qian2021effects}, \citet{bernstein2022contribution}, and \citet{diamond_effects_2019} among others. \citet{phillips_measuring_2020} additionally reports that, relative to 2010 ACS data, Infutor undercounts all state populations, but not by much, and out-of-state movers. A contrasting finding, reported by \citet{diamond_effect_2020}, is that Infutor might overcount the population according to the 2000 Census in San Francisco. Such a finding might be driven by specific spatiotemporal idiosyncrasies of the San Francisco data in 2000, which is not included in the subset we analyze; however, the bulk of the literature, and all the literature which analyzes the same subset of the data we do, is consistent with our finding that Infutor undercounts the data. \citet{diamond_effect_2020} also suggest that Infutor might overcount populations due to lacking information about deaths; this is consistent with our finding that Infutor overcounts the older populations in Figure \ref{fig:biases}\textbf{c}.

In Figure \ref{fig:biases}, we also assess whether under- or over-represents demographic subpopulations\footnote{Prior to conducting this assessment, we scale the Infutor population to match the overall population, so any discrepancies are not caused merely by overall undercounting}. \citet{ramiller_residential_2024} similarly study representation biases of Infutor in King County, Washington, during the 2015-2019 5-year period. They find that Infutor undercounts the county population while overrepresenting White, older, home-owning, and high-income populations. Later, they regress population errors in tract-level demographics to find that Infutor records are overrepresented in areas with higher White and high-income populations among other characteristics. We confirm most of their findings in this limited spatiotemporal scale at national level. However, the authors use the NARC3 dataset---a subset of Infutor's address records that contains detailed demographic information---and thus, beyond the spatiotemporal scope, our analyses might be substantially different. 

\subsection{Assessment of additional demographic biases}
\label{SI:validation-biases-additional}

\begin{figure}[h!]
	\centering
\includegraphics[width=\textwidth]{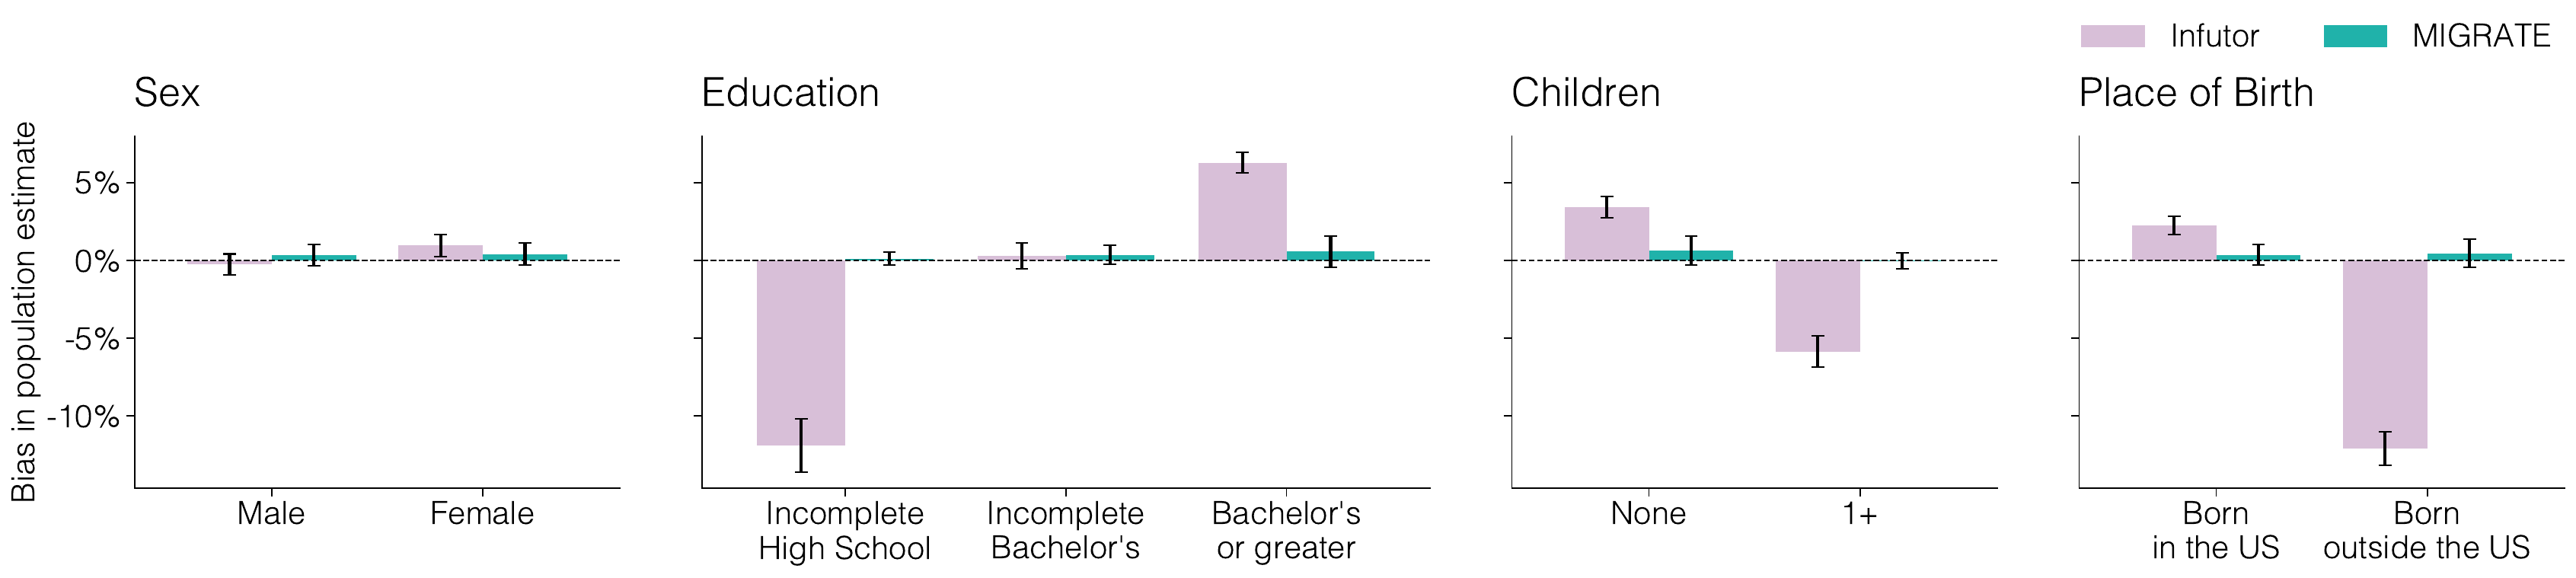}
	\caption{\textbf{Additional analysis of socioeconomic and demographic biases at CBG population level.} Variables are taken from the 5-year ACS CBG estimates. Bias is averaged over $n=5$ population data releases (American Community Survey 5-year estimates, 2015 through 2018) Error bars represent standard deviations across these releases.}
    \label{fig:biases-extra}
\end{figure}

We documented biases in the Infutor dataset geographically (Figure \ref{fig:biases}\textbf{a}) and along the dimensions of urbanization, age, race, household tenure, and poverty (Figure \ref{fig:biases}\textbf{c}). Here, we provide additional analyses of demographic bias by sex, educational attainment, number of children per household, and country of birth (Supplementary Figure \ref{fig:biases-extra}). We find that Infutor displays negligible bias on the basis of sex. However, Infutor underrepresents populations with less formal education while overrepresenting populations with more formal education. Populations living in households with no children are overrepresented while those in households with children are underrepresented. This finding is consistent with the Infutor data documentation, which describes a lack of records for people under the age of 18 (therefore, children will be undercounted). Infutor also undercounts foreign-born residents by about 12\%. \ourdataset essentially eliminates biases along all these demographic dimensions.

\paragraph{Biases in Representation of Immigrant Populations}

Because of our finding that Infutor undercounts the foreign-born population, and previous research hypothesizing that Infutor may undercount undocumented immigrants specifically~\citep{downes2023can, bernstein2022contribution, phillips_measuring_2020}, we conduct further analyses investigating Infutor's representation of undocumented immigrants. Infutor draws from many data sources --- including cell phone bills, phone books, credit header files, public government records, property deeds, county property records, vehicle warranties, and data from vehicle repair and maintenance providers \cite{diamond_effects_2019, phillips2024homelessness, boar2023consumption} --- and some of these sources may contain data for undocumented immigrants. There were an estimated 11 million undocumented immigrants in the United States in the 2018-2022 period, about 27\% of the estimated foreign-born population \citep{baker_estimates_2024}. 

To measure the biases of Infutor in representing the undocumented immigrant population, we investigate whether the relative population error correlates with estimates of the undocumented population. We use data on the yearly undocumented population per state provided by the Pew Research Center \citep{passel_what_2024}, which is the most granular data available. As expected from the results in Figure \ref{fig:biases}\textbf{a}, which documents bias in Infutor data at the county level, there is geographic bias in the Infutor data at the state level as well. Infutor undercounts the population in states with larger proportions of undocumented immigrants: there is a Spearman correlation of $\rho=-0.401$ between the state-level Infutor error and the proportion of undocumented immigrants per state, averaging across the decade (Supplementary Figure \ref{fig:biases-undocumented}\textbf{b}).

\begin{figure}[htb!]
	\centering
\includegraphics[width=\textwidth]{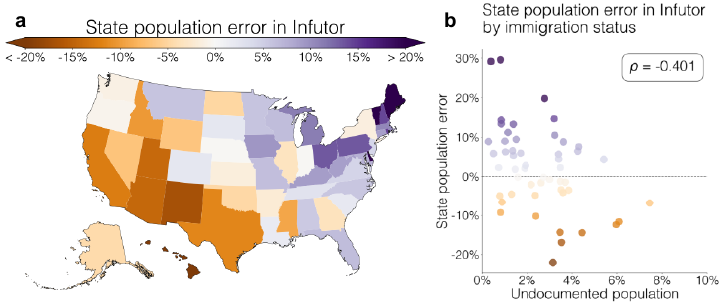}
	\caption{\textbf{Infutor undercounts the undocumented immigrant population.} We study the representation of the undocumented immigrant population by Infutor at the state level. \textbf{(a)} Average errors in state populations in Infutor data relative to Census data. \ourdataset estimates remove all state-level errors by construction. \textbf{(b)} Spearman correlation between the estimated share of undocumented immigrants in the state population (x-axis) and error in Infutor population estimates (y-axis). Infutor is more likely to undercount states with larger proportions of undocumented immigrants.}
    \label{fig:biases-undocumented}
\end{figure}

Importantly, as with other demographic biases in the Infutor dataset, harmonizing the dataset with Census data reduces biases with respect to immigrant populations as well. Census statistics do include undocumented immigrants \citep{us_census_bureau_about_2025}, and so rescaling to match Census populations will mitigate Infutor's biases.\footnote{However, Census data may also be imperfect with respect to its coverage of undocumented migrants if they are, for example, less likely to respond to surveys.} In particular, \ourdataset corrects all bias at state level by construction. As shown in Supplementary Figure \ref{fig:biases-extra}, \ourdataset also significantly reduces the bias for the overall foreign-born population.
