# Supplementary material for: Inferring fine-grained migration patterns across the United States
Source: arXiv:2503.20989 source file (2026-01-07)
Supplement: Supplementary file 3 [file A2_national.tex]

\section{Additional analyses of national migration}
\label{SI:socioeconomic-trends}

In this section we provide additional analyses of national migration trends to complement the findings of Section \ref{sec:national}.

\subsection{Out-migration rates by CBG type}

\begin{table}[h!]
    \centering
    \begin{tabular}{|r|r|c|c|}
            \hline 
        &
        & \textbf{Out-migration rate (per 1,000)}
        & \textbf{Out-movers} \\
        \hline
        \textbf{Plurality Race} & White & 132 & 31,425,400 \\
        &Black & 128 & 3,823,677 \\
        &Asian & 124 & 889,755 \\
        &Hispanic & 118 & 5,289,710 \\
        \hline
        \textbf{Urbanization}&Urban & 135 & 35,481,142 \\
        & Rural & 104 & 5,947,401 \\
        \hline
    \textbf{Income Quartile}&Bottom & 130 & 8,621,155\\
    &2nd& 130 & 9,944,217\\
&3rd& 131 & 11,011,339 \\
&Top& 128 & 11,851,831 \\
        \hline
    \end{tabular}
    \captionsetup{width=\textwidth}
    \caption{\textbf{Stratified out-migration.} Out-migration rates (per 1,000 people) and raw counts of out-movers categorized by plurality race, urbanization level, and income quartile. We average the values across all years in the period.}
    \label{tab:outmigration_by_group}
\end{table}

Supplementary Table \ref{tab:outmigration_by_group} reports the average out-migration rates for each of the ten CBG groups we analyze in the main text. The average out-migration rate in all CBGs is $13.0\%$, with $0.9\%$ standard deviation across years. Out-migration rates are lower in plurality Hispanic and rural CBGs; out-migration rates remain similar across income quartiles.

\subsection{Additional statistics on migration homophily}
\label{SI:socioeconomic-homophily}

\begin{figure}[h!]
	\centering
    \includegraphics[width=\textwidth]{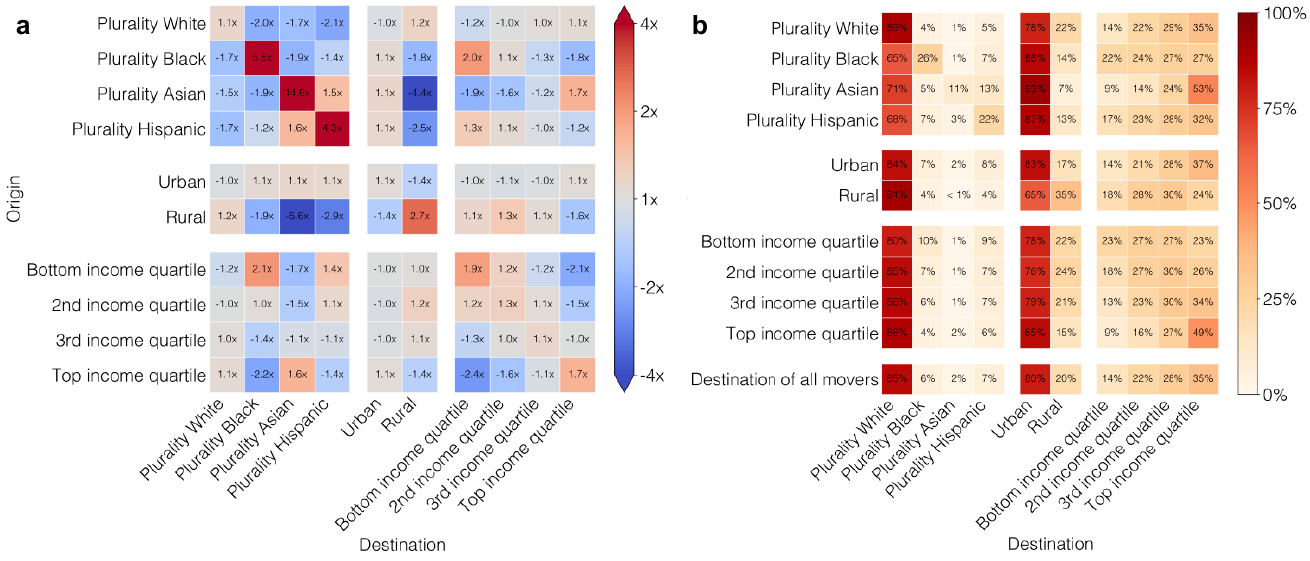}
	\caption{\textbf{Additional national migration statistics.} \textbf{(a)} Flows between the ten types of CBGs discussed in the main text relative to the share of all movers who moved to CBGs in the particular group. Each cell reports the ratio $\frac{\text{share of movers from origin CBG group moving to destination CBG group}}{\text{share of all movers moving to destination CBG group}}$; for example, the top left value of $1.1\times$ reports the ratio of the share of movers from plurality white CBGs who move to plurality white CBGs (90\%) to the share of movers from all CBGs who move to plurality white CBGs (80\%). \textbf{(b)} Flows between the ten types of CBGs discussed in the main text when restricting to out-of-county movers demonstrate that homophily persists for long-distance moves.}
    \label{fig:SI:homophily}
\end{figure}

In Supplementary Figure \ref{fig:SI:homophily}, we extend the analysis of national homophily patterns in migration documented in Figure \ref{fig:national_migration}\textbf{a}. Supplementary Figure \ref{fig:SI:homophily}\textbf{a} shows the shares of movers moving between groups of CBGs relative to the share of all movers who move to that group of CBGs (that is, a version of Figure \ref{fig:national_migration}\textbf{a} where the value in each cell is divided by the corresponding value in the row `Movers from all CBGs').

Homophily in migration might occur because many moves are local (within county or within 5 miles) and demographics are spatially correlated. To investigate this possibility, we restrict our analysis to out-of-county moves in Figure Supplementary \ref{fig:SI:homophily}\textbf{b}. Absolute racial homophily is less prominent---i.e. there are smaller shares in the diagonal of the race by race submatrix---yet still present: out-of-county movers from plurality Black, Asian, and Hispanic CBGs are 4.3$\times$, 5.5$\times$, and 3.1$\times$ likelier than out-of-county movers as a whole to move to CBGs with the same plurality race group (vs. 5.5$\times$, 14.6$\times$, and 4.3$\times$ for all movers).

\subsection{Additional statistics on economic mobility in migration}
\label{SI:socioeconomic-income}

\begin{figure}[b]
	\centering
    \includegraphics[width=.9\textwidth]{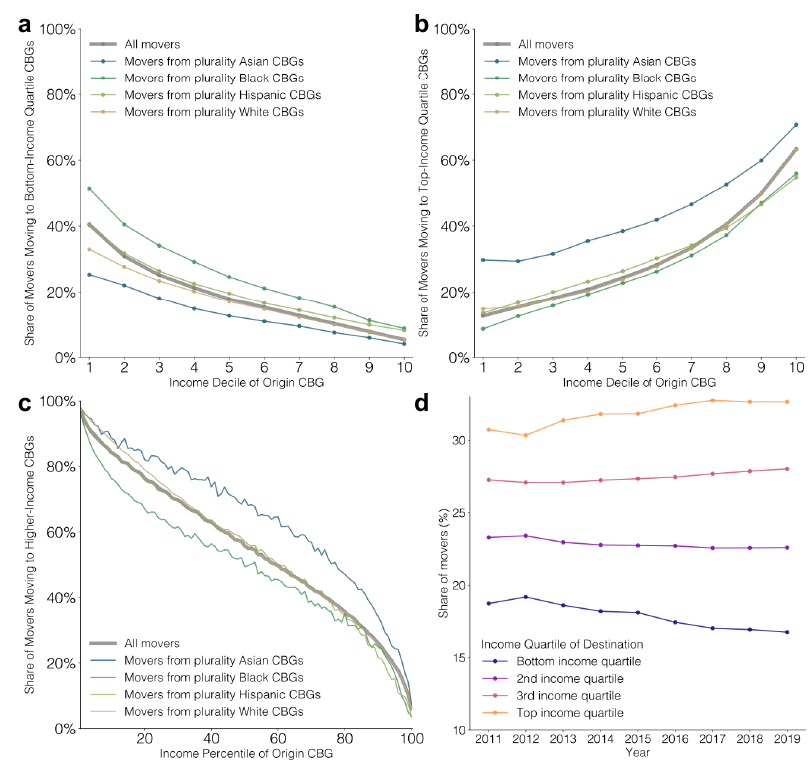}
	\caption{\textbf{Further national migration statistics on upwards mobility.} Probability of moving to a \textbf{(a)} top-income quartile CBG, \textbf{(b)} bottom-income quartile CBG, and \textbf{(c)} higher-income CBG conditioned on current residence median income and plurality race. In \textbf{(c)}, we classify current residence CBGs by income percentiles as opposed to deciles (as in the main text). Disparities remain robust. \textbf{(d)} Movers remain more likely to move to top-income-quartile CBGs than bottom-income-quartile CBGs throughout the decade, with the disparity increasing in magnitude over time.} \label{fig:SI:income_pct}
\end{figure}

Supplementary Figure \ref{fig:SI:income_pct} provides additional analyses supporting our finding of racial disparities in economic mobility (Figure \ref{fig:national_migration}\textbf{b}): movers from plurality Asian CBGs are more likely than movers as a whole, and movers from plurality Black CBGs less likely, to move to higher-income CBGs, even when controlling for income of origin CBG. We show that analogous racial disparities still emerge when looking at probability of moving to a CBG in the top income quartile (Supplementary Figure \ref{fig:SI:income_pct}\textbf{a}) or bottom income quartile (Supplementary Figure \ref{fig:SI:income_pct}\textbf{b}) as opposed to the probability of moving to a higher-income CBG (as in the main text). These disparities also emerge when controlling for origin CBG income percentile (Supplementary Figure \ref{fig:SI:income_pct}\textbf{c}), as opposed to decile, as in the main text. We also observe that the gap in upward mobility widens during the decade: the share of movers going to a top income quartile CBG increases from 31\% to 33\% while the share of movers going to a bottom income quartile CBG decreases from 19\% to 17\% (Supplementary Figure \ref{fig:SI:income_pct}\textbf{d}); overall, the ratio of out-movers moving to top income quartile versus bottom income quartile CBGs increases from 1.64 to 1.95.

\subsection{Additional statistics on moving distance}
\label{SI:socioeconomic-geography}

\begin{figure}[h!]
	\centering
    \includegraphics[width=\textwidth]{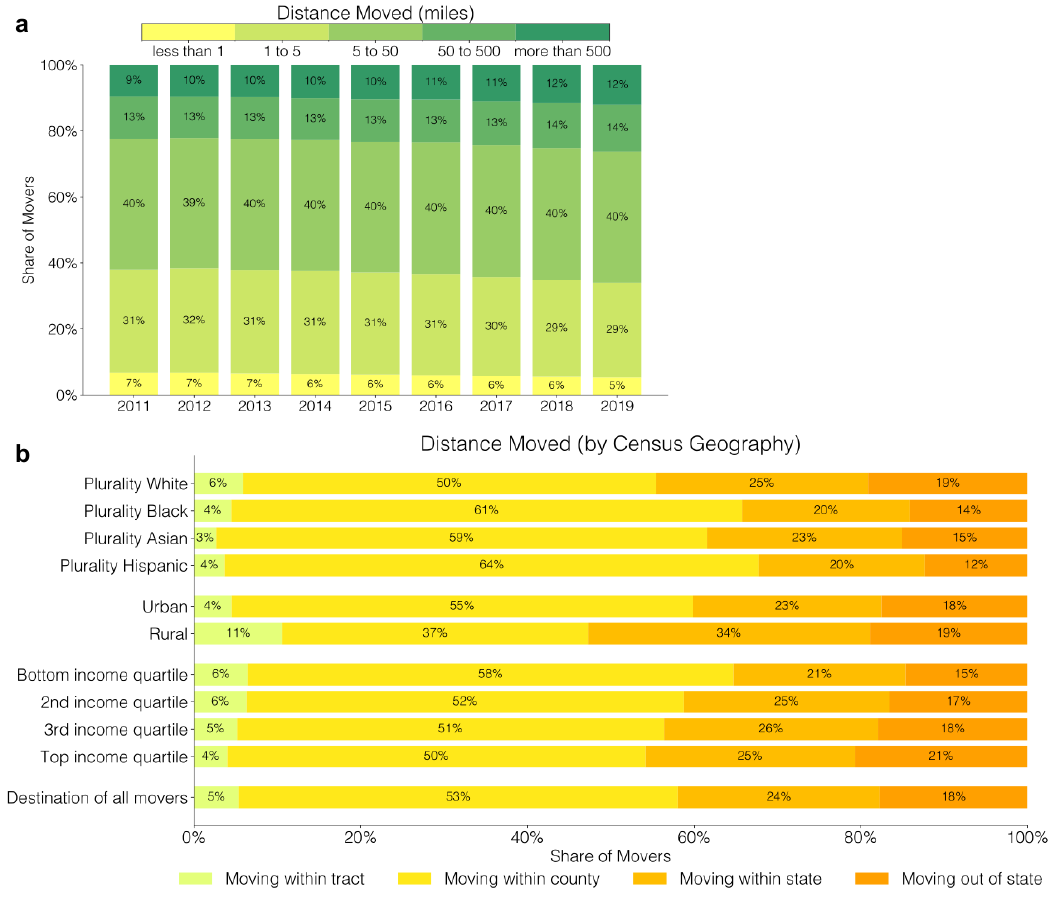}
	\caption{\textbf{Further national migration statistics on distance moved.} \textbf{(a)} Moving distance by year.  \textbf{(b)} Fraction of movers moving within tract, county, and state.}
    \label{fig:SI:distance-moved}
\end{figure}

Supplementary Figure \ref{fig:SI:distance-moved} provides additional statistics on moving distance, expanding the findings in Figure \ref{fig:national_migration}\textbf{c}. Supplementary Figure \ref{fig:SI:distance-moved}\textbf{a} reports how moving distance changes over time, showing a general increase over the decade: the share of movers moving over 50 miles, for example, grows from about 22\% to about 26\%, and the average moving distance increases from 154 to 191 miles in the decade. Supplementary Figure \ref{fig:SI:distance-moved}\textbf{b} reports moving distance stratified by geographic boundary (that is, the share of movers remaining within tract, county, and state). Findings are generally consistent with those reported in Figure \ref{fig:national_migration}\textbf{c}, and also with published ACS figures, which state that over half of moves happen within counties \cite{kerns-damore_migration_2023}.
