# Supplementary material for: Inferring fine-grained migration patterns across the United States
Source: arXiv:2503.20989 source file (2026-01-07)
Supplement: Supplementary file 4 [file A3_local.tex]

\section{Additional case studies of local migration patterns}
\label{SI:cases}

In this section we provide two case studies of how \ourdataset reveals policy-relevant local migration patterns absent from publicly available data in New York City: a study of socioeconomic disparities on out-mover destinations, and a description of migration patterns to and from public housing buildings.

\subsection{Destinations of New York City outmovers}
\label{SI:cases-income}

\begin{figure}[htb!]
	\centering
\includegraphics[width=0.8\textwidth]{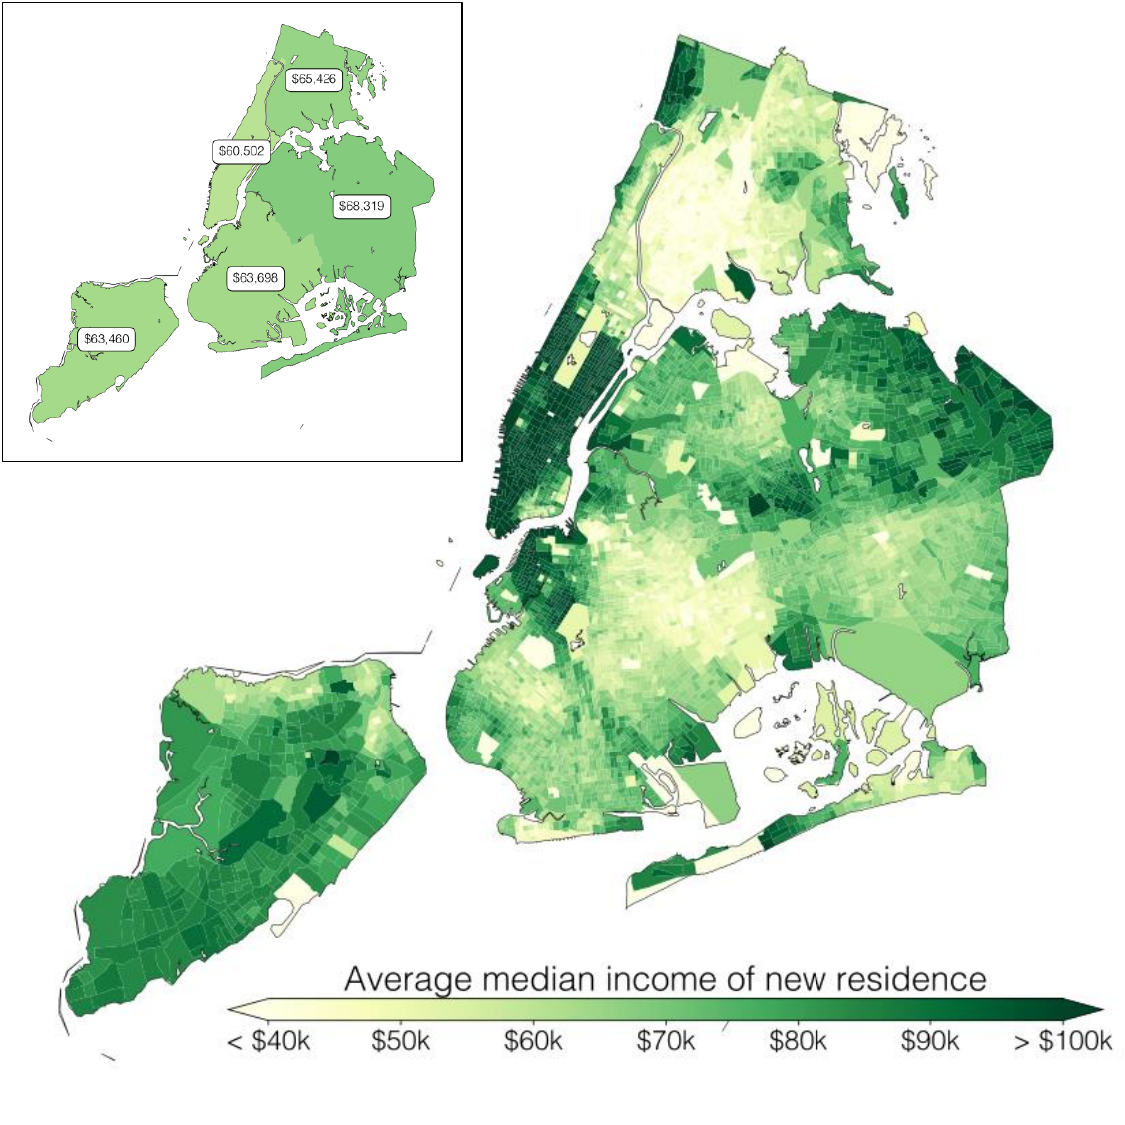}
	\caption{Average income (in US dollars \$) of destination CBGs and counties for New York City out-movers in the 2010-19 period. The large map uses \ourdataset estimates and 5-year ACS CBG data. The inset map shows the corresponding distribution using only publicly available migration data from 5-year ACS county-to-county estimates.}
    \label{fig:income}
\end{figure}

We provide a case study contrasting \ourdataset with publicly available county-to-county migration data when analyzing migration stratified by a demographic or socioeconomic feature. Supplementary Figure \ref{fig:income} plots the average income of the CBG to which a person moves according to their previous CBG of residence. To compute this quantity for a given CBG $i$, we average the mean income of all destination CBGs $j$ for out-movers of CBG $i$ weighted by the number of out-movers from $i$ to $j$. We perform an analogous computation for the county plot in the inset.

Comparing these results to the data available at county level reveals striking within-county variation. For example, the average income of the county to which people from Manhattan moved was $\$82,934$---lower than that of the other four counties in New York City. \ourdataset reveals, however, that movers from some CBGs in Manhattan moved to areas with the highest average income among all New York City CBGs --- above $\$175,000$ at times --- while movers from other Manhattan CBGs moved to areas with some of the lowest average incomes. Intra-county socioeconomic differences factor heavily in out-migration: Manhattan out-movers with the highest-income destinations tended to reside in the central and lower parts of the county (which tend to have higher incomes), whereas those with lower-income destinations came mostly from northern CBGs (which tend to have lower incomes). Similar within-county dynamics occur in the other four counties. Overall, this analysis illustrates the important demographic heterogeneity in migration which is concealed at the county level.

\subsection{New York City Housing Authority}
\label{SI:cases-NYCHA}

\begin{figure}[htb!]
	\centering
\includegraphics[width=\textwidth]{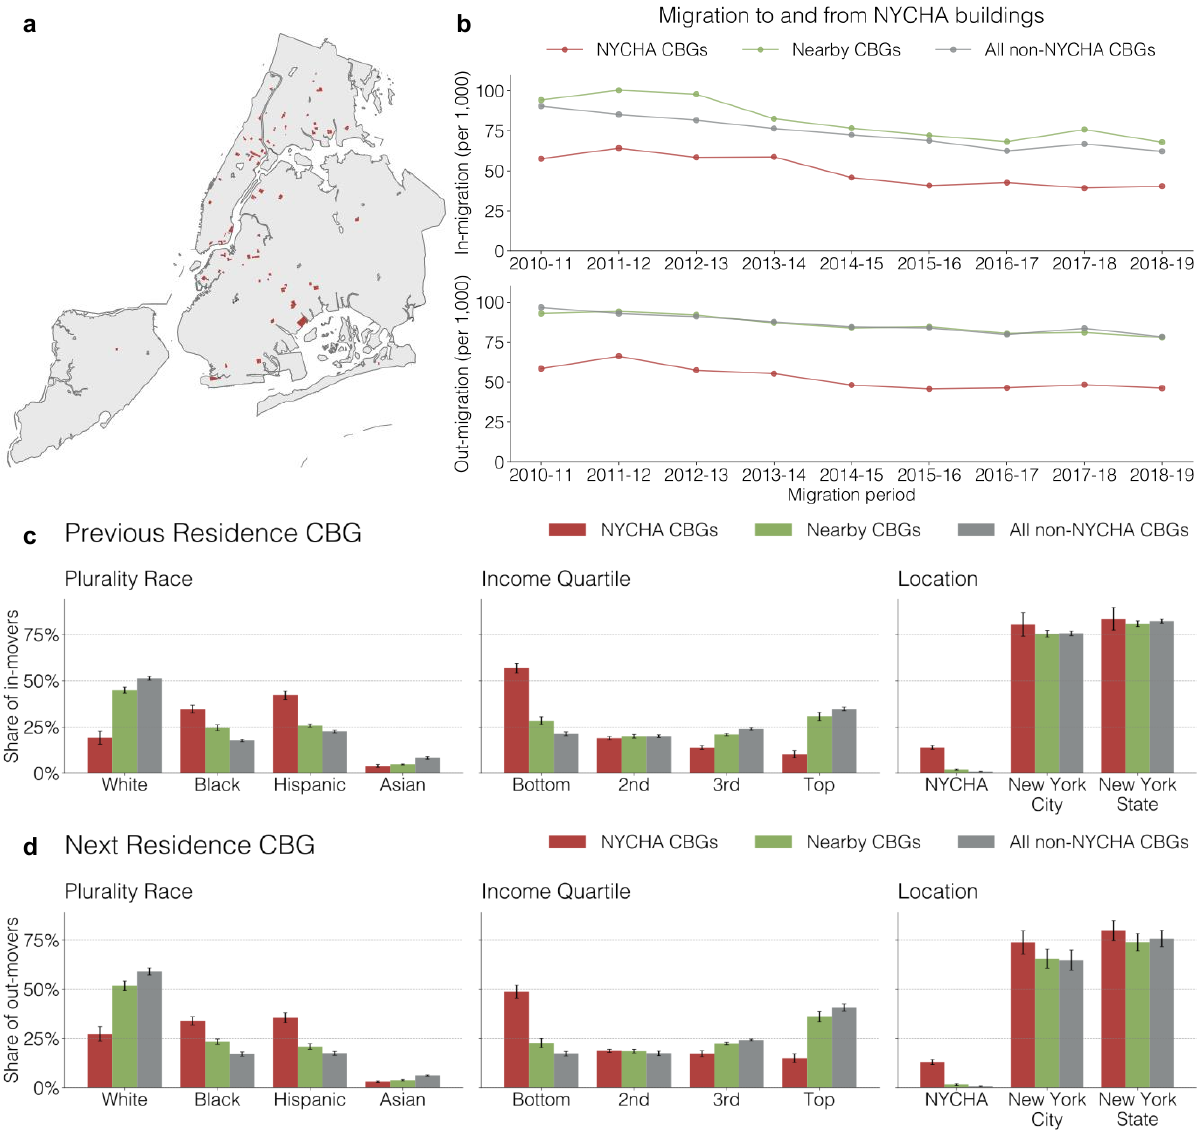}
	\caption{We use \ourdataset to understand migration to and from New York City Housing Authority (NYCHA) developments. \textbf{(a)} A map of the 114 Census Block Groups (marked in red) where all residential units are owned by NYCHA (i.e., where all the population lives in a NYCHA development). \textbf{(b)} Time series of in- and out-migration rates for NYCHA CBGs (red line), as well as for CBGs nearby (within 250 meters of a NYCHA development; green line) and non-NYCHA CBGs within New York City (gray line). NYCHA CBGs have consistently lower in- and out-migration rates, implying a less mobile population. \textbf{(c)} Demographics of previous residence CBG for in-movers into NYCHA buildings as well as for the other CBG groups considered, aggregated across the decade (error bars represent standard deviation across years). \textbf{(d)} Demographics of next residence CBG for out-movers.}
    \label{fig:NYCHA}
\end{figure}

Ensuring that residents have access to affordable housing is an important and challenging policy goal \cite{favilukis2023affordable}. One way of achieving this is through the creation and management of public housing units: for example, the New York City Housing Authority (NYCHA) is the largest public housing authority in the US, providing affordable housing to over 500,000 authorized residents \cite{nycha_factsheet_2024}. We provide a case study illustrating how the \ourdataset dataset can be used to understand which residents make use of public housing units, thereby illuminating the effect of this component of affordable housing policy.

We identify all 114 New York City Census Block Groups whose residential units are entirely owned by NYCHA using New York City's Primary Land Use Tax Lot Output (PLUTO) dataset \cite{nyc_pluto} (Supplementary Figure \ref{fig:NYCHA}\textbf{a}). We compare migration patterns for these CBGs, which we refer to as ``NYCHA CBGs'', to migration patterns of two other groups of non-NYCHA CBGs: (i) nearby CBGs (within 250 meters of a NYCHA development) and (ii) all non-NYCHA CBGs in New York City.\footnote{We excluded from the analysis all 345 CBGs (about 5.3\% of all New York City CBGs) where some but not all of the residential units are owned by NCYHA.} NYCHA CBGs have had consistently lower in-migration and out-migration rates than the two comparison groups of CBGs throughout the decade (Supplementary Figure \ref{fig:NYCHA}\textbf{b}), implying a less mobile population. This is consistent with prior findings that residents of public housing and recipients of rental benefits have longer tenancies than average New York City residents~\cite{nycha_factsheet_2024,chen_measuring_2023}. %NYCHA reports that the average public housing resident tenancy length is 26.3 years \cite{nycha_factsheet_2024}, while researchers have found that the average tenancy in non-rent stabilized apartments is around 5.8 years \cite{chen_measuring_2023}.

To get a sense of the residents being served by NYCHA and their migration trajectories, we examine the demographics of the CBGs where NYCHA in-movers move from (Supplementary Figure \ref{fig:NYCHA}\textbf{c}) and where NYCHA out-movers move to (Supplementary Figure \ref{fig:NYCHA}\textbf{d}). Compared to non-NYCHA in-movers, NYCHA in-movers are likelier to move from plurality Black or Hispanic CBGs, as well as bottom income quartile CBGs. The same is true of NYCHA out-movers: they are also more likely to move to plurality Black or Hispanic CBGs, and bottom-income-quartile CBGs, than are non-NYCHA out-movers. The CBGs that NYCHA movers move to are higher-income than the CBGs they move from, providing evidence of upward mobility. NYCHA out-movers are also more upwardly mobile than non-NYCHA movers: 82\% of NYCHA out-movers move to CBGs of higher median income, compared to 55\% of all non-NYCHA out-movers.

We also quantify whether NYCHA in-movers and out-movers move within NYCHA, within New York City, and within New York State. There is a significant amount of shuffling within the NYCHA system: 14\% of in-movers to a NYCHA CBG came from another NYCHA CBG, and 13\% of out-movers from a NYCHA building go to another NYCHA CBG. This shuffling may be due in part to mandated renovations or building closures that result in temporary resident relocations by NYCHA \cite{navarro_harlem_2014, fernandez_new_2010, zaveri_improve_2023}. On average across the decade that we study, NYCHA out-movers are likelier than non-NYCHA movers to remain within New York City (74\% vs. 65\%); however, this gap has decreased in recent years.

Overall, this analysis highlights how \ourdataset can provide insights into which residents are served by public housing policy. Beyond this case study of New York City, this approach could be extended to study public housing in other cities, or to study the effects of public housing foreclosures---which has been a topic of interest among other migration researchers \cite{phillips_measuring_2020}.
