# Supplementary material for: Inferring fine-grained migration patterns across the United States
Source: arXiv:2503.20989 source file (2026-01-07)
Supplement: Supplementary file 5 [file A4_privacy.tex]

\section{Privacy Protections}
\label{SI:privacy}

In this section we detail the measures we took to preserve the privacy of individuals in the \ourdataset data release. Analysis of the Infutor dataset was determined to be not human subjects research by the Cornell Institutional Review Board (IRB \#0145225).

First, in contrast to the original Infutor data, the data we release is aggregated: it contains only estimated migration between CBG-CBG pairs, and no information about individuals. This level of data aggregation is consistent with other data sources which have been made available to researchers. For example, mobility data often contains the aggregate counts of individuals moving from a given CBG to a given point of interest on a given day \cite{abbiasov202415, chang2021mobility, kostandova2024systematic, xu2025using, yabe2024behaviour}.

Second, the matrices we release are probabilistic and rescaled: in particular, the fact that a particular entry of the CBG-CBG migration matrix is non-zero does not guarantee that a given number of individuals moved between those CBGs (or indeed, that any did at all). This is because individuals are mapped probabilistically to CBGs (e.g., if we have only a ZIP code for an individual, they are mapped probabilistically to CBGs within that ZIP code) and the migration matrices are rescaled multiple times. 

Third, we release the data only to researchers for non-profit use who agree to a data use agreement pledging not to re-identify individuals in the data, and to adhere to privacy-protecting measures when storing data and presenting results, following manual review of their application and research project.

Finally, we compute the average number of destinations (unique CBGs) for out-movers from each CBG. The purpose of the analysis is to assess how difficult it would be to track a given individual if one knew they lived in a given CBG and then moved. Across CBGs and years, the mean number of destinations for outmovers is $272.2$ (median $234$). We redact from the public data release migration information for the very small proportion of CBGs ($0.558\%$) for which 90\% of out-movers travel to 10 or fewer CBGs. All analyses in the paper were conducted with the full data.
